# Supplementary material for: Towards a Sustainable Microgrid on Alderney Island Using a Python-based Energy Planning Tool
Source: arXiv:2007.15165 source file (2020-07-30)
Supplement: Supplementary file 1 [file IET-Conference-Paper-Additional-Information.pdf]

# Additional Information

## I) <u>Submission Specification for Conference Papers</u>

This 'Submission Specification for Conference Papers' document provides instructions for the submission of Conference Papers for publication on the IET Digital Platform.

This document is to be used in conjunction with the 'Manuscript-template.docx'.
**The Conference Paper is to be prepared in MS Word format and then printed to PDF.**

### 1. Submission requirements

Conference papers must satisfy the following requirements:

### 1.1 Manuscript Submission

**1.1.1 Originality**: Is the work scientifically rigorous, accurate and novel? Does the work contain significant additional material to that already published? Has its value been demonstrated?

**1.1.2 Plagiarism**: All conference papers submitted to the IET for publication must record original work which has not been published previously. Any alleged cases of plagiarism will be dealt with according to the 'IET Policy in Relation to Plagiarism, Infringement of Copyright and Infringement of Moral Rights and Submission to Multiple Publications'.

**1.1.3 Multiple submissions:** The IET does not permit manuscripts included in its conference proceedings to be simultaneously under review for another conference or publication.
Once a case of multiple submissions has been established, the paper/s in question will be immediately declined for publication by the IET.

**1.1.4 Relevance:** Is the material appropriate to the scope of the conference to which it is submitted?

**1.1.5 Clarity:** Is the English clear and well written? Poorly written English may obscure the scientific merit of your paper. Are the ideas expressed clearly and concisely? Are the concepts understandable?

### 2. Post-print Policy

2.1.1 The author may post post-prints of their conference papers published by the IET on repositories, servers and websites of any sort, provided that these servers are operated by the author's institution or the funding body contributing to the research. To comply with funding requirements, authors may also deposit their conference papers in repositories (or mirror sites) designated by the funding body.

The conditions attached to this are as follows:

2.1.2 Access to such servers is not for commercial use and does not depend on payment of access, subscription, or membership fees.

2.1.3 The following wording clearly appears on the front page of the post-print:

"This paper is a post-print of a paper submitted to and accepted for publication in Conference Proceedings of *conference title* and is subject to Institution of Engineering and Technology Copyright. The copy of record is available at IET Digital Library"

2.1.4 The post-print must be the author's version and not the IET version/PDF.

2.1.5 The post-print must not be posted prior to publication of the paper by the IET and when posted any preprint version should be removed.

### 3.1 Copyright

3.1.1 An author submitting a paper should ensure that he or she has the right to publish the paper and that it contains nothing defamatory. The IET will assume that all co-authors have agreed to the submission of any paper received.

3.1.2 Your conference paper must be accompanied by a signed licence to publish.

3.1.3 Copyright: Unless the paper is either "United Kingdom Crown copyright" or "a work of the US Government and in the Public Domain", the copyright remain with the author(s).

3.1.4 Right to publish: An author submitting a paper should ensure that he or she has the right to publish the paper and that it contains nothing defamatory. The IET will assume that all co-authors have agreed to the submission of any paper received.

### 4.1 Permissions to Reproduce

4.1.1 All authors must secure permission from the copyright holder for reproducing previously published text, figures and tables. The source of the reproduced material must be given in full and the words 'Reproduced by permission of .....' included with the illustration.

## II) PDF format requirement

All PDFs shall be set as follows:

**Version:** Adobe PDF Version 1.5-1.8 (Acrobat 5-8)

**Fonts:** All fonts must be 'embedded subset'.

**Document Properties:**

**Title:** Full title of the paper.
**Authors:** All contributing author names to be included.
**Subject:** Full conference name and abbreviation.
**Keywords:** Keywords as set in the paper at Item 2, Keywords.

## III) IET Digital Library and Inspec Indexing requirements

Papers that will be submitted for publication on the IET Digital Library, and subsequent indexing in Inspec, IEEE Xplore and EI Compendex, must be submitted in the following format:

**All PDFs must** be in the format as specified as stated in Paragraph 2 above (PDF format requirement).
